# Supplementary material for: Wormhole MAML: Meta-Learning in Glued Parameter Space
Source: arXiv:2212.14094 source file (2022-12-28)
Supplement: Supplementary file 1 [file 7_Appendix.tex]

\appendix
\section{Appendix}
\textcolor{blue}{Feel free to remove this section if it's not used in the end.}
